# Supplementary material for: Droplet transport in a nanochannel coated by hydrophobic semiflexible polymer brushes: the effect of chain stiffness
Source: arXiv:1710.02414 ancillary file (2017-10-17)
Supplement: Supplementary file 1 [file sup_mat.pdf]

# Supporting information for: Droplet transport in a nanochannel coated by hydrophobic semiflexible polymer brushes: the effect of chain stiffness

K. Speyer[‡†] and C. Pastorino[†*,‡]

*Departamento de Física de la Materia Condensada, Centro Atómico Constituyentes, CNEA, Av.Gral. Paz 1499, 1650 Pcia. de Buenos Aires, Argentina, and CONICET, Avenida Rivadavia 1917, C1033AAJ Buenos Aires, Argentina*

E-mail: pastor@cnea.gov.ar

## Tracking the droplet's center of mass

Knowing the precise location of the droplet in each time step is crucial to perform averages of quantities that depend on the position of the drop (e.g. liquid velocity, density profiles, brush deformation). Calculating the center of mass of the fluid may give a sensibly different result than calculating the center of mass of the liquid. This is due to the presence of a gaseous phase in coexistence with the liquid phase. To estimate the effect of the vapor in this calculation, we will use typical values adopted in the present work: temperature

*To whom correspondence should be addressed

†Departamento de Física de la Materia Condensada, Centro Atómico Constituyentes, CNEA, Av.Gral. Paz 1499, 1650 Pcia. de Buenos Aires, Argentina

‡CONICET, Avenida Rivadavia 1917, C1033AAJ Buenos Aires, Argentina

$T = 0.8\varepsilon/k_B$, channel length $L = 322\sigma$, number of liquid particles $n_l = 4000$ . The ratio of gas particles $n_v$ over liquid particles $n_l$ is roughly

$$\frac{n_v}{n_l} = \frac{\rho_v V_v}{\rho_l V_l} \approx \frac{\rho_v (L - D)}{\rho_l D} = 0.42\,,$$

where $L$ is the length of the simulation box in the flow direction, $D$ is the droplet extension in the flow direction, and $\rho_l$ and $\rho_v$ are the liquid and vapor phase densities of the Lennard-Jones fluid. This means that 30% of the particles are in the gaseous phase, and should not be counted to calculate the droplet's center of mass. If the droplet is at the beginning of the simulation box, averaging the position of the fluid blindly may lead to a mean value outside the liquid phase, as shown in the histogram of Figure S1. The straightforward solution would be to identify all the liquid particles, and take the mean value over this set. However, identifying the particles in the liquid is a very costly algorithm, as it involves a loop over all pairs, and it scales $O(N^2)$ with the number of particles. Considering that the molecular dynamics program scales as $O(N\,logN)$, an order $N^2$ algorithm may slow down the simulations considerably.

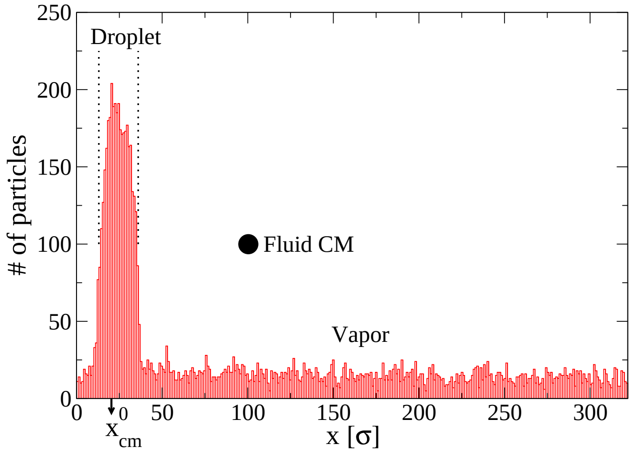


Figure S1: Histogram of particle positions along the channel ($x$ coordinate). The difference in densities between vapor and liquid is clearly appreciated. The fluid's center of mass (black circle) falls outside the droplet, due to the significant number of particles in vapor phase. The mode of the distribution ($x^0_{cm}$) is a better estimator for the droplet's center of mass.

We have developed an efficient ($O(N)$) algorithm to extract the droplet's center of mass,

given the fluid particles positions. First, it is necessary to do a rough estimation of the droplet's position. This can be achieved by doing a histogram of the positions of all fluid particles, as seen in Figure S1, and taking out the mode of the distribution ($x^0_{cm}$). This is the first guess for the center of mass of the liquid. If the droplet size is not known before the beginning of the simulation, it can be also estimated from the histogram. Let $h_{max}$ be the maximum value of the histogram, then there will be at leas one value of $x$ for which $h[x_{start}] < h_{max}/2$ and $h[x_{start}+\Delta x_{bin}] \geq h_{max}/2$. This value $x_{start}$ corresponds to the left end of the droplet. Analogously, there will be at least one value $x_{end}$, for which $h[x_{end}] > h_{max}/2$ and $h[x_{endt}+\Delta x_{bin}] \leq h_{max}/2$, which corresponds to the right end of the droplet. The droplet size can be estimated then as $D = x_{end} - x_{start}$. We proceed then with an iterative approach to the solution. All particle's positions are translated according to $x^{i+1} \rightarrow x^i - x^i_{cm} + L/2$, where $L$ is the length of the simulation box and $i$ is the iteration index. It is necessary to correct for periodic boundary conditions in this step. The idea is that in each successive iteration, the center of mass of the droplet will be closer to the center of the simulation box. Afterwards, a new guess of the center of mass is generated by computing the mean value of the translated coordinates, restricted to a window near the center of the simulation box: $x^{i+1}_{cm} = \langle x^{i+1} \rangle'$. Restricting the volume to compute the new average is a key element in the algorithm, because it allows a strong reduction of the influence of the gas particles in the computation. If the window to compute the new center of mass is chosen correctly, then all the particles in the liquid phase will be counted, and most of the particles in the vapor phase will be left out, thus achieving a more accurate estimate in each step. In this case the window to calculate the new center of mass was chosen as $L/2 - D < x < L/2 + D$. With a new guess of the center of mass another iteration is performed, in the same way as described above. It is important to observe that $x_{cm} = L/2$ is a fixed point of the algorithm, i.e. if the iteration starts with the droplet in the center of the simulation box, then the new guess will be $x^{i+1}_{cm} = x^i_{cm} = L/2$, and the procedure is converged. For starting values $x^0_{cm} \neq L/2$, the algorithm converges towards $\lim_{i\rightarrow\infty} x^i_{cm} = L/2$. To compute the center of mass of the

liquid droplet after $j$ iterations, the used formula is $x_{cm} = L/2 + \sum_{i=0}^{j} (x^i_{cm} - L/2)$. The total number of iterations to be performed depends on the precision desired in the final result. The criteria taken in this work are $|x^i_{cm} - L/2| < D/200$ and $|x^i_{cm} - L/2| \leqslant |x^{i-1}_{cm} - L/2|$. The first criterion gives the desired precision in terms of the droplet's size. The second one warrants that the correction in the last iteration is smaller than that of the previous iteration. This is important when working with periodic boundary conditions. The typical number of iterations used in this work is 8 and the droplet center of mass was located with a precision of $0.1\sigma$

There exists another fixed point, if half of the droplet is on the right corner, and the other half is on the left corner of the simulation box. Fortunately this is not a problem, because this fixed point is unstable. If the starting guess for the center of mass of the droplet is $x^0_{cm} = L/2$, then the algorithm will converge to the stable solution, finding correctly the position of the center of mass of the droplet. In this case the second criterion of convergence is necessary, to ensure that the fixed point is the correct one.

The advantages of this tracking algorithm are that it is fast $O(N)$, the precision can be tuned, and it is trivial to generalize it for n-dimensions. A downside is that it does not support multiple droplet detection in the same simulation box. Although a modified version of this algorithm can handle this situation.

# Setting the appropriate channel width via least squares

The problem consist in selecting the optimum value of channel width $L_z$ to obtain a droplet as similar as possible to a reference droplet. This is not trivial, because the polymer brush height is strongly dependent on the local stiffness of the individual polymers and studying the droplet's flow properties as a function of chain stiffness is one of our key goals in this work. The idea is keeping constant the effective channel width and the droplet's shape for all the studied cases. To select the value of $L_z$, the two-dimensional density histograms of

the droplets are compared to the reference droplet via least squares: $\chi^2 = \sum_{bins}(\rho_{Lz} - \rho_{ref})^2$. In Figure S2, the value of $\chi^2$ is plotted against the channel width $L_z$, for polymers of rigidity $l_p/l_c = 11$. The value of $L_z$ that corresponds to a minimum of the $\chi^2$ function is selected. The distance between walls is chosen to obtain similar droplets' shapes for all the explored bending rigidities.

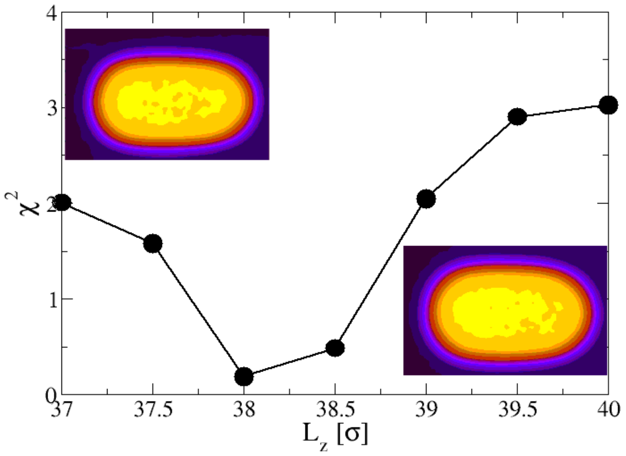


Figure S2: To select the appropriate width of the channel ($L_z$), the 2 dimensional density histograms of the droplets are compared. This case corresponds to polymers of reduced persistence length $l_p/l_c = 11$. $\chi^2$ is a metric that quantifies the distance between the simulation and the reference droplet, the lower it's value, the more similar the droplets. A value of $\chi^2 = 0$ is achieved for an exact match between histograms. Insets: two-dimensional histograms are presented for the smallest and largest values of $L_z$ explored.
